# Supplementary material for: VINP: Variational Bayesian Inference with Neural Speech Prior for Joint ASR-Effective Speech Dereverberation and Blind RIR Identification
Source: arXiv:2502.07205 source file (2025-09-09)
Supplement: Supplementary file 1 [file 8.Appendix.tex]

\appendices
\section{Proof of the First Zonklar Equation}
Appendix one text goes here.

% you can choose not to have a title for an appendix
% if you want by leaving the argument blank
\section{}
Appendix two text goes here.
